# Supplementary material for: A Theory of Available-by-Design Communicating Systems
Source: arXiv:1611.05651 source file (2016-11-17)
Supplement: Supplementary file 1 [file appendix-definitions.tex]

% \vspace{-1cm}
\section{Additional Definitions}

\subsection{Type System}
\label{app-type-system}
